# Supplementary material for: Twisted phase of the orbital-dominant ferromagnet SmN in a GdN/SmN heterostructure
Source: arXiv:1504.04425 source file (2015-04-17)
Supplement: Supplementary file 1 [file supplemental_material_submit.pdf]

## Supplemental Material: Twisted phase of the orbital-dominant ferromagnet SmN in a GdN/SmN heterostructure

## SI. ADDITIONAL SPECTRA

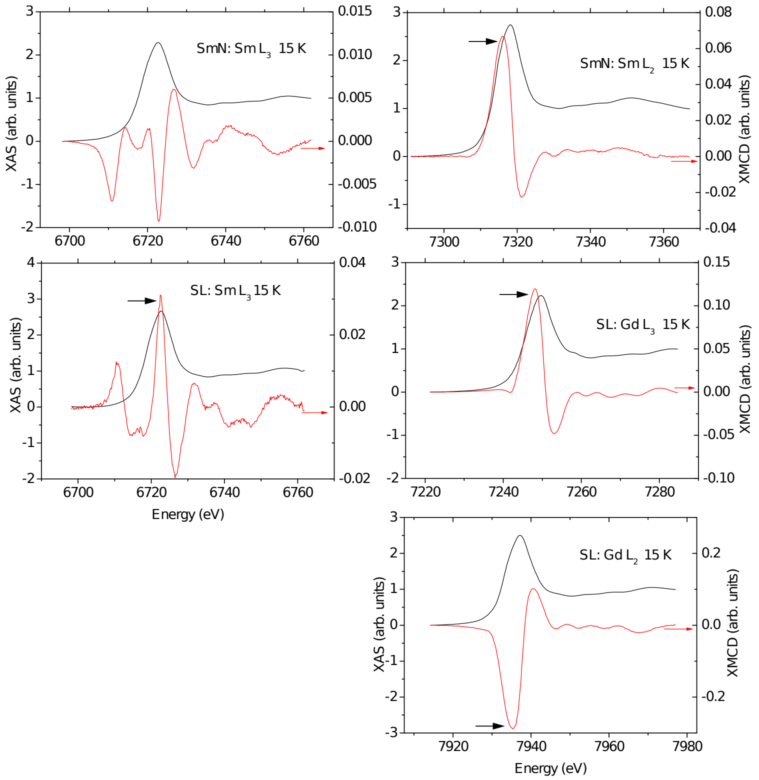


FIG. S1: L-edge XAS and XMCD for the SmN and SmN/GdN superlattice samples taken at 15 K and in a field of 6 T at grazing incidence. The hysteresis and temperature dependence were found by following the most prominant feature in the XMCD spectra (black arrows).

## SII. DETAILS OF THE MODEL

The modelling of the twisted phase uses the results of Goto *et al.*[1], who consider an exchange spring system in a one-dimensional continuum model with nearest neighbor exchange, Zeeman coupling, and interfacial pinning of the soft layer spins at the interface. We adapt the model to SmN by incorporating the orbitally dominant net moment into the Zeeman term, and an out-of-plane orientation of the applied magnetic field $H$ and GdN spin-moments, which are assumed parallel to $H$ at fields $\geqslant 2$ T. Out of plane rotation (i.e. the plane formed by $H$ and the moments)

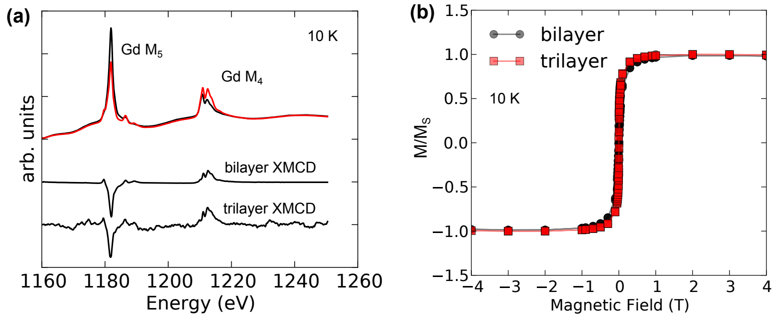


FIG. S2: (a) Gd $M_{4,5}$-edge XAS for the bilayer and XMCD for the bilayer and trilayer at 4 T and 10 K. The large background in the absorption spectra is due to EXAFS at the Ga $L_{2,3}$-edges from the GaN capping layers. (b) SQUID magnetization measurements for bilayer and trilayer at 10 K with field in plane.

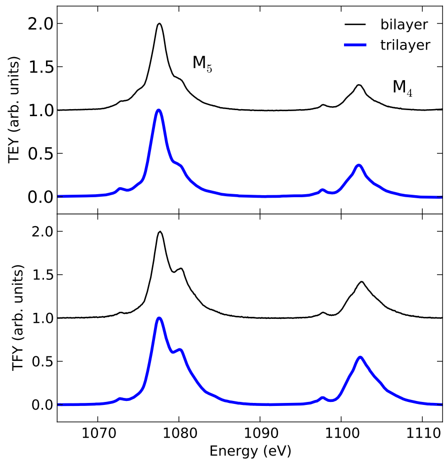


FIG. S3: Sm M-edge XAS spectra in TEY and TFY modes for the bilayer and trilayer with the background subtracted and normalized for comparison.

can be safely ignored as this creates a static field which tends to only increase the energy. The minimization of the total energy functional shown in equation (1) leads to the depth profile of the spin moment $\mu_S$ (and hence the orbital moment $\mu_L$ and net moment $\mu$):

$$\theta(z) = 2 \arcsin \left[ K^{-1} (\alpha d) \, \mathrm{sn} \, (\alpha z) \right] , \tag{S1}$$

where $\alpha = \sqrt{H M_S / 2A}$, and the functions $K^{-1}$ and sn are the inverse of the complete elliptic function of the first kind and the Jacobi elliptic function of the first kind, respectively. The boundary conditions were chosen such that $\theta(d) = 0$ (Sm spin is aligned with the Gd spin at the

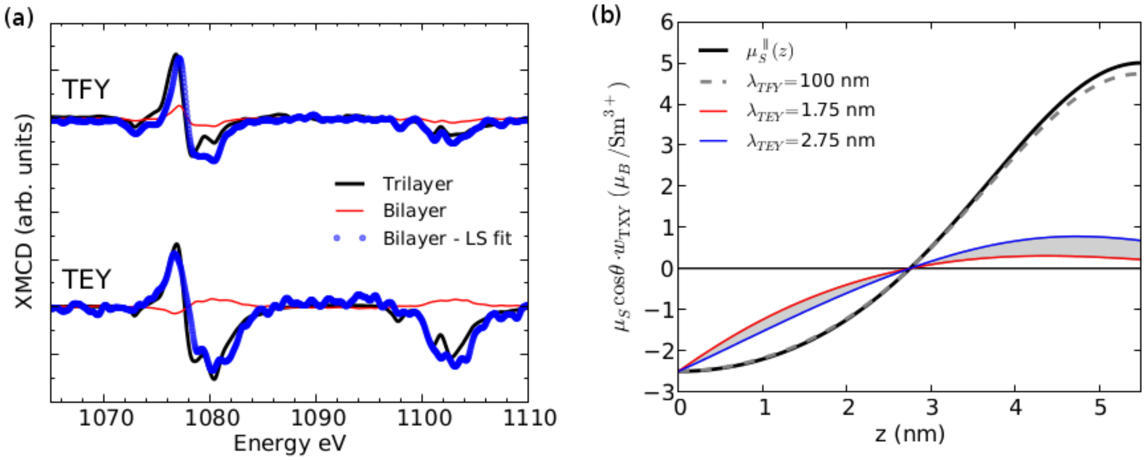


FIG. S4: (a) The least-squares fit of the bilayer spectra to the trilayer spectra. The circles represent the bilayer spectrum multiplied by the fit value $R_{\mathrm{TXY}}$. (b) A plot of $\mu_S \cos\theta(z) w_{\mathrm{TXY}}$ (where $w_{\mathrm{TXY}} = \exp(-z/\lambda_{\mathrm{TXY}})$) for various values of $\lambda_{\mathrm{TXY}}$ ($\mu_S^{\parallel}$ corresponds to $\mu_S \cos\theta(z)$) as a function of depth through the SmN film, with the GdN interface at $z = 5.5$ nm.

SmN-GdN interface) and $d\theta(z)/dz|_{z=0} = 0$ (SmN free surface). This equation has a solution only when the condition $H \geqslant \pi^2 A/2d^2 M_s$ is met. The input parameters to calculate $R_{\mathrm{TXY}}$ were taken from the experimental results, with $H = 4$ T, $d = 5.5$ nm, $M_s = 0.035$ $\mu_B$/Sm$^{3+}$ per unit cell, and $J_{\mathrm{ex}}$ estimated from the known paramagnetic Curie temperature of 27 K according to the mean-field Heisenberg relationship $J_{\mathrm{ex}} = \frac{3}{2n}\frac{k_B T_c}{S(S+1)} = 0.033$ meV, where $n = 12$ corresponds to the 12 nearest Sm$^{3+}$ neighbors in the fcc lattice[2,3]. The exchange stiffness $A = 4J_{ex}S^2/a^*$ then depends on the SmN $4f$ ground state spin value of $S = 5/2$ and nearest neighbor Sm$^{3+}$ distance $a^*$, related to the SmN lattice constant by $a^* = a/\sqrt{2}$. We note the factor $(g-1)$, where $g$ is the Landé factor, should be included if an orbital moment is present, however this cancels out in the calculation of $A$.

As stated in the main text, the large $\lambda_{\mathrm{TFY}} \sim 100$ nm probing depth in the TFY is large enough to fully probe the SmN film, $R_{\mathrm{TFY}}$ is insensitive to the precise value of this parameter. Using the above paramaters results in a value of $R_{\mathrm{TFY}} = -0.11$, within the error of the experimental value $-0.12 \pm 0.02$. For the TEY ratio, we calculate $R_{\mathrm{TEY}} = 0.24$ for $\lambda_{\mathrm{TEY}} = 1.75$ nm and $R_{\mathrm{TEY}} = 0.19$ for $\lambda_{\mathrm{TEY}} = 2.25$ nm. The experimental value of $R^{\mathrm{exp}}_{\mathrm{TEY}} = 0.20$ thus corresponds to the value of $\lambda_{\mathrm{TEY}} \sim 2.15$ nm, which is on the order expected[4,5]. The least-squares fit of the XMCD spectra which yields the experimental $R$-values is shown in Fig. S4 (a). The resulting spin-moment depth profiles calculated using $J_{\mathrm{ex}} = 0.033$ meV are shown in Fig. S4 (b), where

$\mu_S \cos\theta(z) \exp(-z/\lambda_{TXY})$ is plotted as a function of depth for the various $\lambda_{\mathrm{TXY}}$ values, along with the actual spin moment profile, $\mu_S(z) \cos\theta(z)$.

---

[1] E. Goto, N. Hayashi, T. Miyashita, and K. Nakagawa, J. Appl. Phys. **36**, 2951 (1965).

[2] C. Meyer, B. J. Ruck, J. Zhong, S. Granville, A. R. H. Preston, G. V. M. Williams, and H. J. Trodahl, Phys. Rev. B **78**, 174406 (2008).

[3] J. B. Goodenough *et al.*, *Magnetism and the chemical bond*, Vol. 98 (Interscience Publishers New York, 1963).

[4] B. T. Thole, G. van der Laan, J. C. Fuggle, G. A. Sawatzky, R. C. Karnatak, and J.-M. Esteva, Phys. Rev. B **32**, 5107 (1985).

[5] J. Stöhr and H. C. Siegmann, *Magnetism: from fundamentals to nanoscale dynamics*, Vol. 152 (Springer, 2007).
